# Supplementary material for: How does the Combined Risk Affect the Performance of Unsupervised Domain Adaptation Approaches?
Source: arXiv:2101.01104 source file (2020-12-30)
Supplement: Supplementary file 1 [file v1_7_appendix.tex]

\section{Proofs of Theorems}
\subsection{Proof of Theorem 1}
Theorem 1 is a corollary of Theorem 2. If we set the transformation space $\mathcal{G}=\{\mathbf{I}\}$, where $\mathbf{I}$ is the identity map from $\mathcal{X}$ to $\mathcal{X}$, then Theorem 1 can be concluded by Theorem 2 directly.
\subsection{Proof of Theorem 2}
Using triangle inequality of $\ell$, we have
\begin{equation}\label{proofTh1}
\begin{split}
& R_t^{\ell}(\mathbf{C}\circ \mathbf{G})\leq R_t^{\ell}(\mathbf{C}^\prime\circ \mathbf{G},\mathbf{C}\circ \mathbf{G})+R_t^{\ell}(\mathbf{C}^\prime\circ \mathbf{G}), 
\\ &
R_s^{\ell}(\mathbf{C}^\prime\circ \mathbf{G},\mathbf{C}\circ \mathbf{G})\leq R_s^{\ell}(\mathbf{C}^\prime\circ \mathbf{G})+R_s^{\ell}(\mathbf{C}\circ \mathbf{G}),
\end{split}
\end{equation}
where ${\mathbf{C}}^\prime$ is any scoring function in $\mathcal{H}$.

%We note that 
%\begin{equation}\label{7}
%\mathbb{Q}^t(U,y|y\in \mathcal{Y}^s)=\left\{
%\begin{aligned}
%\begin{split}
%&~~~~~~~~~~~0, ~~~{\rm if}~y=c+1;\\
%&\frac{\mathbb{Q}^t(U|y)\mathbb{Q}^t(y)}{1-\pi_{C+1}^t},  ~~~{\rm if}~y \in \mathcal{Y}^s,
%\end{split}
%\end{aligned}
%\right.
%\end{equation}
% where $U\subset \mathcal{X}$ is any $P_{X^t}{\rm -measurable}$ set.
 Above inequalities imply that
 \begin{equation}\label{theorem2inequ2}
 \begin{split}
 & R_t^{\ell}(\mathbf{C}\circ \mathbf{G})-R_s^{\ell}(\mathbf{C}\circ \mathbf{G}) 
 \\\leq & R_t^{\ell}(\mathbf{C}^\prime\circ \mathbf{G},\mathbf{C}\circ \mathbf{G})-R_s^{\ell}(\mathbf{C}^\prime\circ \mathbf{G},\mathbf{C}\circ \mathbf{G})\\ +& R_s^{\ell}(\mathbf{C}^\prime\circ \mathbf{G})
 +R_t^{\ell}(\mathbf{C}^\prime\circ \mathbf{G}).
 \end{split}
 \end{equation}
 
According to inequality (\ref{theorem2inequ2}), it is easy to check that
\begin{equation*}
 \begin{split}
 & R_t^{\ell}(\mathbf{C}\circ \mathbf{G})-R_s^{\ell}(\mathbf{C}\circ \mathbf{G}) 
 \\\leq & \sup_{\mathbf{C},\mathbf{C}^\prime \in \mathcal{H}}\big | R_t^{\ell}(\mathbf{C}^\prime\circ \mathbf{G},\mathbf{C}\circ \mathbf{G})-R_s^{\ell}(\mathbf{C}^\prime\circ \mathbf{G},\mathbf{C}\circ \mathbf{G}) \big |\\ +& \min_{\mathbf{C}^\prime\in \mathcal{H}} \big ( R_s^{\ell}(\mathbf{C}^\prime\circ \mathbf{G})
 +R_t^{\ell}(\mathbf{C}^\prime\circ \mathbf{G}) \big )
 \\\leq & d_{\mathcal{H}}^{\ell}(P_{\mathbf{G}(X_s)},P_{\mathbf{G}(X_t)})\\ +& \min_{\mathbf{C}^\prime\in \mathcal{H}} \big ( R_s^{\ell}(\mathbf{C}^\prime\circ \mathbf{G})
 +R_t^{\ell}(\mathbf{C}^\prime\circ \mathbf{G}) \big ).
 \end{split}
 \end{equation*}

 %Based on (\ref{Th6}), (\ref{Th7}), (\ref{Th8}) and the definition of the discrepancy distance, we have
% \begin{equation*}
% \begin{split}
 %     ~~~&~R_t({\bm h}\circ {\bm T}_t)-R_s({\bm h}\circ {\bm T}_s)\\{\leq}&R_t(\overline{{\bm h}}\circ {\bm T}_t)+R_s(\overline{{\bm h}}\circ {\bm T}_s)+\left|\int_{\mathcal{X}\times \mathcal{Y}} \ell({\bm h}({\mathbf{x}}),\overline{{\bm h}}({\mathbf{x}})){\rm d} P_{{\bm T}_t(X_t)}({\mathbf{x}})-\int_{\mathcal{X}\times \mathcal{Y}} \ell({\bm h}({\mathbf{x}}),\overline{{\bm h}}({\mathbf{x}})){\rm d}P_{{\bm T}_s(X_s)}({\mathbf{x}})\right|\\\leq&\Lambda(\overline{{\bm h}},{\bm T}_s,{\bm T}_t)+d_{{\bm h},\mathcal{H}}^{\ell}(P_{{\bm T}_t(X_t)},P_{{\bm T}_s(X_s)})
  %    .
 %     \end{split}
% \end{equation*}
% Hence,
%\begin{equation}\label{Th15}
% \begin{split}
 %    &R_t({\bm h}\circ {\bm T}_t)-R_s({\bm h}\circ {\bm T}_s)\leq \min_{\overline{{\bm h}}\in \mathcal{H}}\Lambda(\overline{{\bm h}},{\bm T}_s,{\bm T}_t)+d_{{\bm h},\mathcal{H}}^{\ell}(P_{{\bm T}_t(X_t)},P_{{\bm T}_s(X_t)})
%      .
 %     \end{split}
% \end{equation}
{The proof has been completed.}

\subsection{Proof of Theorem 3}
   \noindent \textbf{Step 1}. 
 \begin{equation*}
 \begin{split}
     &R_s^{\ell}(\mathbf{C}_t\circ \mathbf{G})+R_t^{\ell}(\mathbf{C}_s\circ \mathbf{G})+\delta \\= & \big( R_s^{\ell}(\mathbf{C}_t\circ \mathbf{G})+R_t^{\ell}(\mathbf{C}_t\circ \mathbf{G}) \big )+\big (R_s^{\ell}(\mathbf{C}_s\circ \mathbf{G})+R_t^{\ell}(\mathbf{C}_s\circ \mathbf{G}) \big)\\  \geq & 2\min_{\mathbf{C}^\prime\in \mathcal{H}}\big( R_s^{\ell}(\mathbf{C}^\prime\circ \mathbf{G}\circ \mathbf{G})+R_t^{\ell}(\mathbf{C}^\prime\circ \mathbf{G}\circ \mathbf{G}) \big)= 2\lambda^{\ell}(\mathbf{G}).
     \end{split}
 \end{equation*}
\noindent  \textbf{Step 2}.  
According to Theorem 2, if we set $\mathbf{C}=\mathbf{C}_s$, we have
\begin{equation}\label{Lab1}
    R_t^{\ell}(\mathbf{C}_s\circ \mathbf{G})\leq R_s^{\ell}(\mathbf{C}_s\circ \mathbf{G})+d_{\mathcal{H}}^{\ell}( {P}_{\mathbf{G}({X}_s)}, {P}_{\mathbf{G}({X}_t)})+\lambda^{\ell}(\mathbf{G})
      .
\end{equation}
If we exchange the source domain and the target domain, then we use Theorem 2 and set $\mathbf{C}=\mathbf{C}_t$. We have
\begin{equation}\label{Lab2}
R_s^{\ell}(\mathbf{C}_t\circ \mathbf{G})\leq R_t^{\ell}(\mathbf{C}_t\circ \mathbf{G})+d_{\mathcal{H}}^{\ell}( {P}_{\mathbf{G}({X}_s)}, {P}_{\mathbf{G}({X}_t)})+\lambda^{\ell}(\mathbf{G})
      .
\end{equation}
Combining the inequality (\ref{Lab1}) and the inequality (\ref{Lab2}), we have
\begin{equation*}
   R_t^\ell(\mathbf{C}_s\circ \mathbf{G})+R_s^\ell(\mathbf{C}_t\circ \mathbf{G}) \leq \delta +2d_{\mathcal{H}}^{\ell}( {P}_{\mathbf{G}({X}_s)}, {P}_{\mathbf{G}({X}_t)}) +2\lambda^{\ell}(\mathbf{G}).
\end{equation*}
Combining the results of \textbf{Step 1} and \textbf{Step 2},
we have proved the result.

\subsection{Proof of Theorem 4}
Using triangle inequality of $\ell_s,\ell_t$, we have
\begin{equation*}
\begin{split}
& R_t^{\ell_t}(\mathbf{C}\circ \mathbf{G})\leq R_t^{\ell_t}(\mathbf{C}^\prime\circ \mathbf{G},\mathbf{C}\circ \mathbf{G})+R_t^{\ell_t}(\mathbf{C}^\prime\circ \mathbf{G}), 
\\ &
R_s^{\ell_s}(\mathbf{C}^\prime\circ \mathbf{G},\mathbf{C}\circ \mathbf{G})\leq R_s^{\ell_s}(\mathbf{C}^\prime\circ \mathbf{G})+R_s^{\ell_s}(\mathbf{C}\circ \mathbf{G}),
\end{split}
\end{equation*}
where ${\mathbf{C}}^\prime$ is any scoring function in $\mathcal{H}$.

The above inequalities imply that
 \begin{equation}\label{theorem4inequ2}
 \begin{split}
 & R_t^{\ell_t}(\mathbf{C}\circ \mathbf{G})-R_s^{\ell_s}(\mathbf{C}\circ \mathbf{G}) 
 \\\leq & R_t^{\ell_t}(\mathbf{C}^\prime\circ \mathbf{G},\mathbf{C}\circ \mathbf{G})-R_s^{\ell_s}(\mathbf{C}^\prime\circ \mathbf{G},\mathbf{C}\circ \mathbf{G})\\ +& R_s^{\ell_s}(\mathbf{C}^\prime\circ \mathbf{G})
 +R_t^{\ell_t}(\mathbf{C}^\prime\circ \mathbf{G}).
 \end{split}
 \end{equation}

 According to inequality (\ref{theorem4inequ2}), it is easy to check that
\begin{equation*}
 \begin{split}
 & R_t^{\ell_t}(\mathbf{C}\circ \mathbf{G})-R_s^{\ell_s}(\mathbf{C}\circ \mathbf{G}) 
 \\\leq & \sup_{\mathbf{C}^\prime \in \mathcal{H}}\big ( R_t^{\ell_t}(\mathbf{C}^\prime\circ \mathbf{G},\mathbf{C}\circ \mathbf{G})-R_s^{\ell_s}(\mathbf{C}^\prime\circ \mathbf{G},\mathbf{C}\circ \mathbf{G}) \big )\\ +& \min_{\mathbf{C}^\prime\in \mathcal{H}} \big ( R_s^{\ell_s}(\mathbf{C}^\prime\circ \mathbf{G})
 +R_t^{\ell_t}(\mathbf{C}^\prime\circ \mathbf{G}) \big )
 \\\leq & d_{\mathbf{C},\mathcal{H}}^{\ell_s\ell_t}(P_{\mathbf{G}(X_s)},P_{\mathbf{G}(X_t)})\\ +& \min_{\mathbf{C}^\prime\in \mathcal{H}} \big ( R_s^{\ell_s}(\mathbf{C}^\prime\circ \mathbf{G})
 +R_t^{\ell_t}(\mathbf{C}^\prime\circ \mathbf{G}) \big ).
 \end{split}
 \end{equation*}
 
{The proof is completed.}
\\\\ 
\section{Additional experimental analysis}
\begin{figure*}[ht]
\centering
\includegraphics[scale=0.45, trim=0 10 0 0, clip]{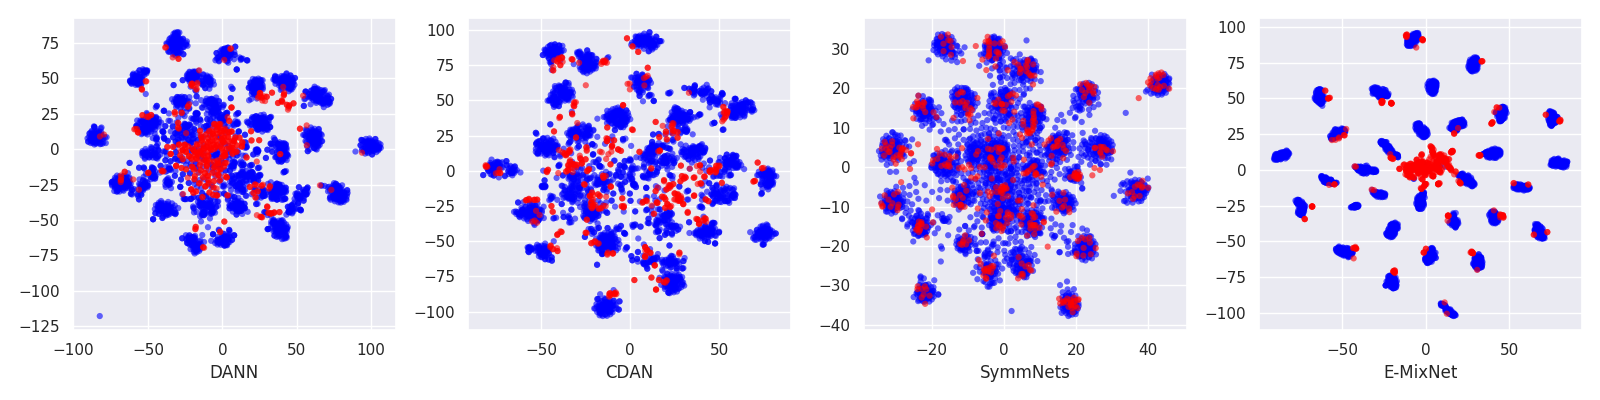}
\caption{Visualization of features}
\label{fig:tsne}
\vspace{-0.5em}
\end{figure*}

\begin{figure}[ht]
\centering
\includegraphics[scale=0.6, trim=0 0 0 0, clip]{alpha.pdf}
\caption{Parameter analysis of $\alpha$}
\label{fig:alpha}
\end{figure}

\textit{Parameter analysis}. Parameter $\alpha$ plays a crucial role in the proxy of combined risk. In this paper, for simplicity, we set $\alpha$ as a fixed value. As shown in Fig. \ref{fig:alpha}, better performance can be achieved when $\alpha$ is set to 0.6. In addition, selecting $\alpha$ in [0.4, 0.6] is recommended.

\textit{Visualization}. To more intuitively demonstrate the efficiency of E-MixNet, we employ t-sne \cite{maaten2008visualizing}, a dimensionality reduction method, to achieve 2D visualization on the task A $\rightarrow$ D on Office-31. As shown as Figure \ref{fig:tsne}, E-MixNet can achieve better performance of distribution alignment. That is because the conditional distribution discrepancy is controlled by the proxy of the combined risk.
